# Supplementary material for: Fairly Allocating Goods in Parallel
Source: arXiv:2309.08685 source file (2023-09-15)
Supplement: Supplementary file 1 [file appendix.tex]

%\section{Preliminaries for parallel computation continued}\label{app: parallel-prelims}

\section{Proofs missing from Section~\ref{sec:verification}}\label{app: missing from verification}

\section{Proofs missing from Section~\ref{sec:ef1 for two and three}}\label{app: missing from two and three agents}

\section{Proofs missing from Section~\ref{sec: matching-revised}}\label{app: matching-revised}

\section{Content missing from Section~\ref{sec: subsidy}\label{app: subsidy}}

\subsection{Proofs missing from Section~\ref{subsec:envy-freeable}}

\subsection{Content missing from Section~\ref{subsec: envy constrained}}\label{app: constrained subsidy}
